# Supplementary material for: Stein Variational Guided Model Predictive Path Integral Control: Proposal and Experiments with Fast Maneuvering Vehicles
Source: arXiv:2309.11040 source file (2024-03-01)
Supplement: Supplementary file 1 [file appendix.tex]

\section{Appendix}

\subsection{Algorithm}
\begin{algorithm}[t]
  \caption{SVG-MPPI}
  \label{alg:SVG-MPPI}
  \begin{algorithmic}[1]
  \Require{Observed state $\myvec{x}_t$, Previous control input sequence $\myarray{U}_{t-1} = \{\hat{\myvec{u}_{\tau}}\}_{\tau=0}^{T-1}$}, Guide particles $\{\myarray{V}_k^g\}_{k=0}^{K_g-1}$
  \Function{Solve}{$\myvec{x}_t$, $\myarray{U}_{t-1}$, $\{\myarray{V}_k^g\}_{k=0}^{K_g-1}$}
    \State{$\myvec{x}_0 \leftarrow \myvec{x}(t)$ }
    \State{/* Transport guide particles */}
    \For{$k \gets 0$ to $K_g$ \textbf{do in parallel}}
        \State{$\tau_k^g \gets \{\myarray{V}_k^g[l]\}_{l=0}^{L-1}$} \Comment{Transportation trajectory}
        \For{$l \gets 1$ to $L$} 
            \State{$\myarray{V}_k^g[l] \gets \myarray{V}_k^g[l-1] + \epsilon \nabla_{\myarray{V}_k^g}\log \mathbb{E}_{\myarray{V}_k^g \sim \mathbb{Q}}[w(\myarray{V}_k^g)]$}
        \EndFor
        \State{$\myarray{V}_k^g \gets \myarray{V}_k^g[L-1]$}
    \EndFor
    \State{/* Pick up a nominal solution $\{\myvec{\Tilde{u}}_{\tau}\}_{\tau=0}^{T-1}$*/}
    \State{$k^* = \text{argmin}_{k}{\{S(\myarray{V}_k^g[L-1])\}}$}
    \State{$\{\myvec{\Tilde{u}}_{\tau}\}_{\tau=0}^{T-1} \gets \myarray{V}^g_{k^*}$} 
    \State{/* Estimate covariance matrix sequence $\boldsymbol{\Sigma}$*/}
    \For{$\tau \gets 0$ to $T$}
        \For{$i \gets 0$ to $m$}
            \State{$\Sigma_{\tau}[i] \gets \text{GauusianFitting}(\tau_{k^*}^g)$}         
        \EndFor
    \EndFor
    \State{$\boldsymbol{\Sigma} = \text{diag}\{\{\Sigma_{\tau}[i]\}_{i=0}^{m-1}\}_{\tau=0}^{T-1}$}
    \State{/* Minimize FKL divergence by MPPI algorithm */}
    \State{Sample $\{\myarray{V}_k\}_{k=0}^{K-1} \sim \myset{N}({U}_{t-1}, \boldsymbol{\Sigma})$}
    \For{$k \gets 0$ to $K$ \textbf{do in parallel}}
        \State{$S(\myarray{V}_k) \gets \text{PredictAndCalcCost}(\myarray{V}_k, \myvec{x}_0)$}
    \EndFor
    \State{$\rho \gets \min_k [S(\myarray{V}_k)]$}
    \State{$\eta \gets \sum_{k=0}^{K-1}\exp(-\frac{1}{\lambda}(S(\myarray{V}_k)-\rho))$}
    \For{$k \gets 0$ to $K$ \textbf{do in parallel}}
        \State{$w_k \gets \eta^{-1} \exp \left( - \frac{1}{\lambda}S(\myarray{V}_k) - \sum_{\tau=0}^{T-1} (\hat{\myvec{u}}_{\tau} - \myvec{\Tilde{u}}_{\tau})^\top \Sigma_{\tau}^{-1} \myvec{v}_{\tau}  \right)$}
    \EndFor
    \State{$\myarray{U}_t = \sum_{k=0}^{K-1}w_k \myarray{V}_{k}$}\\
    \Return{$\myarray{U}_t$}
  \EndFunction
  \end{algorithmic}
\end{algorithm}
